# Supplementary material for: Probabilistic Conceptual Explainers: Trustworthy Conceptual Explanations for Vision Foundation Models
Source: arXiv:2406.12649 source file (2024-10-31)
Supplement: Supplementary file 1 [file X_suppl.tex]

\clearpage
\setcounter{page}{1}

\maketitlesupplementary
\why{remeber to mask out appendix if not finished, and submit a separate file afterwards.}
\hao{TODO for HENGYI: need to add some implementation detail in the Supplement, e.g., what perturbations are used, what code (PyTorch), what learning rate, XX}
% The distribution of the response is a generalized linear model,
% \begin{align}
%     p(y|\z_m, \et, \delta) = h(y,\delta) \exp \{\frac{(\et^T \bar \z_m)y - A(\et^T \bar\z_m)}{\delta}\}
% \end{align}
d
\textbf{Repeated Sampling for Baselines.}
Certain baseline methods, such as those described in~\cite{ribeiro2016lime, lundberg2017shap}, rely on random sampling, resulting in varying explanations for each run. To address this, we execute these baseline methods multiple times, averaging the scores of the each property across all runs. The frequency of these repeated runs is determined by the time required to generate explanations. Aiming for real-world efficiency and effectiveness, we presume the total time for interpreting all dataset samples should not exceed a few days. Considering the time complexity of different baselines, SHAP is executed 100 times, and LIME is run 10 times.

Assuming that the topic of $d'th$ document $\z_d$ subjects to a variational Normal distribution 
$\bar \z_d = \frac{1}{N}\sum_{i=1}^N z_{d,i}$, where $z_{d,i}$ can be approximate by a variational distribution parameterized by $\phi_{d,i}$
\begin{align*}
    q(z_{d,n}|\phi_{d,n}) = \text{Categorical}(z_{d,n}|\phi_{d,n}).
\end{align*}
%which indicates that $z_{d,n} = E[\phi_{d,n}]$.

\subsection{Relevance}
Our model's predict label $y_d$ subjects to a multinomial distribution

\begin{align*}
    p(\y_d|H,\bar \z_d) = \prod_{i=1}^{C}[\frac{\exp(\et_i^T \bar\z_{d})}{\sum_{j}\exp(\et_j^T \bar\z_{d})}]^{y_{d,i}}
\end{align*}
\why{can do SGD(ADAM) on target $\bar y$ }
where $H = [\et_1, \et_2, ..., \et_K]$.

Employing Taylor's expansion, we have
\begin{align*}
    \mathcal{L}_f =& \mathbb{E}_{q(\bar\z)}[\log p(\y_d|\bar\z_d,\H)] \\
     =& \sum_{j=1}^{C} y_{d,j} (\et^T_{j}  \bar \ph_d) 
     -  E_{q(\bar\z)} \log (\sum_{j=1}^{C} \exp (\et^T_{j} \bar\z_d)  ) \\
     \approx & \sum_{j=1}^{C} y_{d,j} (\et^T_{j}  \bar \ph_d) 
     -   \log (\sum_{j=1}^{C} \exp (\et^T_{j} \bar\ph_d + (1/2)\et_j^T\Si_{d}\et_j)  )     
\end{align*}
where
\begin{align} \label{eq:phi_avg}
    \bar \ph_d = \frac{1}{N_d}\sum_n \ph_{d,n}
\end{align}

We can use this $\LM_d$ to perform gradient ascent in differentiable CLDA. 

We can then 

By Taylor's Expansion, we have that
\begin{align}
 \log (\sum_{j} \exp(\a_j^T \x + b_j)) =&  \log (\sum_{j} \exp(\a_j^T \x_0 + b_j)) 
 + (\x - \x_0)^T (\sum_j \exp(\a_j^T \x_0 + b_j) \a_j) / \sum_j \exp(\a_j^T \x_0 + b_j)\nonumber \\
 & + O((\x-\x_0)^T (\x-\x_0))
\end{align}
Taking the fist two terms, we have that
\begin{align}
\log (\sum_{j=1}^{C} \exp (\et^T_{j} \bar\ph_d + (1/2)\et_j^T\Si_{d}\et_j)  )  \approx
\log (\sum_{j=1}^{C} \exp (\et^T_{j} \bar\ph'_d + (1/2)\et_j^T\Si_{d}\et_j)  ) 
+ (\bar\ph_d-\bar\ph'_d) ^T \frac{\sum_{j=1} ^{C} \exp(\et^T_{j} \bar\ph'_d  +(1/2)\et_j^T\Si_{d}\et_j)\et_j} {\sum_{j=1}^{C} \exp (\et^T_{j} \bar\ph'_d + (1/2)\et_j^T\Si_{d}\et_j)},
\end{align}
where $\bar\ph'_d$ is the value of $\bar\ph_d$ at last iteration of coordinate ascent.

Taking the derivative w.r.t. $\ph$, we have that
\begin{align} \label{eq:gradient_phi_classify}
    \frac{\partial \LM_f }{\partial \bar\ph_d} \approx \sum_{j=1}^{C} y_{d,j} \et_j 
    -  \frac{\sum_{j=1} ^{C} \exp(\et^T_{j} \bar\ph'_d + (1/2)\et_j^T\Si_{d}\et_j)\et_j} {\sum_{j=1}^{C} \exp (\et^T_{j} \bar\ph'_d + (1/2)\et_j^T\Si_{d}\et_j)}
\end{align}
%\why{ref https://arxiv.org/pdf/0712.2526.pdf, eq. 26, by ignoring denominator $\sum_{j=1}^{C} \exp (\et^T_{j} \bar\ph_d + (1/2)\et_j^T\Si_{d}\et_j) $.}
%Use first-order gradient Taylor's expension for $\ph_d$. 

%$A + \ph_d \cdot \Delta L/\Delta  \ph_d + O(\ph_d)$
Note that by definition in~\eqnref{eq:phi_avg}, 
\begin{align}
    \frac{\partial \LM_f }{\partial \ph_{dn}} = \frac{\partial \LM_f }{\partial \bar \ph_d} \cdot \frac{\partial \bar\ph_d }{\partial \phi_{dn}} = \frac{1}{N} \frac{\partial \LM_f }{\partial \bar \ph_d}.
\end{align}

%%%%%%%%%%%%%%%%%%%%%%%%%%%%%%%%%%%%%%%%%%%%%%%%%%%%%%%%%%%%%%%%%%%%%%%%%%%%%%%
%%%%%%%%%%%%%%%%%%%%%%%%%%%%%%%%%%%%%%%%%%%%%%%%%%%%%%%%%%%%%%%%%%%%%%%%%%%%%%%
(i) We omit bias using feature augmentation.  (Ref https://arxiv.org/pdf/0712.2526.pdf D0, eq 23)

(ii) We approximate bias term by definition of expectations.

For the Covariance Matrix of $\ph_{d,n}$, which we denote as $\ph_n$:
\begin{align*}
    Cov[z_{d,n}]_{i,j} =& \EB[(\phi_{n,i}-\EB[\phi_{n,i}])
    (\phi_{n,j}-\EB[\phi_{n,j}])]  \\
    =& \EB[(\phi_{n,i}-z_{n,i}) 
    (\phi_{n,j}-z_{n,j})]  \\
    =& \EB[z_{n,i}z_{n,j}] - \phi_{n,i}\phi_{n,j} \\
    =& \begin{cases}
     -\phi_{n,i}\phi_{n,j}, & \text{if }i\neq j \\
     \phi_{n,i} (1-\phi_{n,i}), & \text{if }i = j 
    \end{cases}
\end{align*}

\begin{align*}
    \EB[\bar \z_d] =& \EB[\frac{1}{N} \sum_{n=1}^{N} z_{d,n}] \\
    =& \frac{1}{N} \sum_{n=1}^{N} \EB[z_{d,n}]\\
    =& \EB[\bar \ph_d]
\end{align*}

\begin{align*}
    \Si_{d} = Cov[\bar \z_d] = & Cov[\frac{1}{N} \sum_{n=1}^{N} z_{d,n}] \\
    = & \frac{1}{N} \sum_{n=1}^{N}Cov[z_{d,n}]
\end{align*}

\subsection{Stability}
(train with contrastive loss, test via simplified L2/cov distances. Training directly with a MSE loss will lead to mode collapse!)

%Define $\mathbb{D}_{-d} \subset \mathbb{D} \backslash \{d\}$.
The Learning objective of contrastive loss can be formulated as follows:
\begin{align*}
 \LM_s =    \mathcal{L}(\bet,\bar \z_d, \bar \z'_d, \bar \z_{f}) = 
    \EB_{q(\bar\z)} \log\frac{\exp(\bet^T (\bar\z_{d}\cdot\bar\z'_{d}))}{\sum_{f\in \mathbb{D}} \exp(\bet^T (\bar\z_{d}\cdot\bar\z_{f}))}           
\end{align*}

where we use element-wise product.

%For implementation, ref SimCLR \hyperlink{https://uvadlc-notebooks.readthedocs.io/en/latest/tutorial_notebooks/tutorial17/SimCLR.html}.

$\bet$ can be either (1) learned jointly (2) fixed to $\1$ (equivalent to inner product)
, we test which config improve the stability metric. 

where $\z'_d$ refers to the augmented data $\z_d$, and $\z_{-d}$ refers to other documents other than $\z_d$.

Expand $\LM$ and notice cross terms in expectations

Assume $z_d, z'_d, z_f$ are independent to simplify.
\begin{align*}
    \LM_s   =&  \bet^T  \bar \ph_d \bar\ph'_d
     -  E_{q(\bar\z)} \log (\sum_{f\in \DB} \exp (\bet^T \bar\z_d\bar\z_f)  ) \\
     \approx & \bet^T  \bar \ph_d \bar\ph'_d
     -   \log (\sum_{f\in \DB}\exp (\bet^T(\bar\ph_d\bar\ph_f )+ (1/2)\bet^T\Si_{s}\bet)  )     
\end{align*}

\begin{align}
    \frac{\partial \LM_s }{\partial \bar\ph_d} \approx \bet^T \bar \ph'_d  - \frac{\sum_{f\in \DB_{-d}}\exp (\bet^T  (\bar \ph_d\bar\ph_f)  ) \cdot \bet^T \bar\ph_f} {\sum_{f\in \DB_{-d}}\exp (\bet^T (\bar\ph_d\bar\ph_f ))}
\end{align}

\begin{align}
    \frac{\partial \LM_s }{\partial \bar\ph_f} \approx  - \frac{\exp (\bet^T  (\bar \ph_d\bar\ph_f)  ) \cdot \bet^T \bar\ph_d} {\sum_{g\in \DB_{-d}}\exp (\bet^T (\bar\ph_d\bar\ph_g ))}
\end{align}
Here we omit $\Si_s$ because by the Lemma below we have that $\Vert (\Si_s)_{ij} \Vert \leq \frac{1}{N^2}$, where $N>100$ in our setting.

Since $\bar z_d, \bar z_f$ are independent, $\EB[\bar z_d \bar z_f] = \EB[\bar z_d]\EB[\bar z_f]$ (cov not zero because of dimensional corr!)

\textbf{Lemma:} compute Cov by definition (Note that this is not a categorical distribution, not sum up to 1. )

\begin{align}\label{eq:cov_z_mul}
    Cov[\bar z_{d} \bar z_f]_{i,j} =& \EB[(\bar z_{di} \bar z_{fi}-\EB[\bar z_{di} \bar z_{fi}])(\bar z_{dj} \bar z_{fj}-\EB[\bar z_{dj} \bar z_{fj}])]  \\
    =& \EB[(\bar z_{di} \bar z_{fi}-\EB[\bar z_{di}]\EB[ \bar z_{fi}]])(\bar z_{dj} \bar z_{fj}-\EB[\bar z_{dj}]\EB[ \bar z_{fj}]])]  \\
    =& \EB[(\bar z_{di} \bar z_{fi}-\bar \phi_{di}\bar \phi_{fi})(\bar z_{dj} \bar z_{fj}-\bar \phi_{dj}\bar \phi_{fj})]  \\
    = & \EB[\bar z_{di} \bar z_{fi}\bar z_{dj} \bar z_{fj}] - \bar\phi_{dj}\bar \phi_{fj}\EB[\bar z_{di} \bar z_{fi}] - \bar\phi_{di}\bar \phi_{fi}\EB[\bar z_{dj} \bar z_{fj}] + \bar\phi_{di}\bar \phi_{fi}\bar\phi_{dj}\bar \phi_{fj} \\
    = & \EB[\bar z_{di} \bar z_{dj}] \EB[\bar z_{fi} \bar z_{fj}] - \bar\phi_{di}\bar \phi_{fi}\bar\phi_{dj}\bar \phi_{fj} \\
\end{align}

\textbf{Case (1): $i=j$}

Then we have that
\begin{align}
    Cov[\bar z_{d} \bar z_f]_{i,j}  = & \EB[\bar z_{di}^2] \EB[\bar z_{fi} ^2] - \bar\phi_{di}^2\bar\phi_{fi}^2 \\
    =& \bar\phi_{di}^2\bar\phi_{fi}^2 - \bar\phi_{di}^2\bar\phi_{fi}^2 \\
    =& 0.
\end{align}

\textbf{Case (2): $i\neq j$}

We notice that
\begin{align}
    \bar z_{di} \bar z_{dj} = \frac{1}{N} \sum_n z_{dni}\cdot  \frac{1}{N} \sum_n z_{dnj} 
\end{align}

And we have that 
\begin{align}
    z_{dni} * z_{dnj} = 0
\end{align}
when $i\neq j$.
Hence,
\begin{align}
    \EB[\bar z_{di} \bar z_{dj}] = & \EB[\bar z_{di}]\EB[\bar z_{dj}] - \frac{1}{N^2} (\sum_{n=1}^N \EB[z_{dni}]\EB[z_{dnj}]) \\
    = & \bar \phi_{di}\bar \phi_{dj} - \frac{1}{N^2} \sum_{n=1}^N \phi_{dni}\phi_{dnj}.
\end{align}

Therefore,
\begin{align}
    Cov[\bar z_{d} \bar z_f]_{i,j} =& (\bar \phi_{di}\bar \phi_{dj} - \frac{1}{N^2} \sum_{n=1}^N \phi_{dni}\phi_{dnj})
    (\bar \phi_{fi}\bar \phi_{fj} - \frac{1}{N^2} \sum_{n=1}^N \phi_{fni}\phi_{fnj})
    \nonumber\\
    &- \bar\phi_{di}\bar \phi_{fi}\bar\phi_{dj}\bar \phi_{fj} \nonumber\\
    = &  \frac{1}{N^4} \sum_{n=1}^N \phi_{dni}\phi_{dnj}\sum_{n=1}^N \phi_{fni}\phi_{fnj}.
\end{align}

Hence, the partial derivative of ELBO w.r.t. $\ph$ is 
\begin{align}
    \frac{\partial \LM }{\partial \ph_{nk}}
    =& \frac{\partial \LM_{u} }{\partial \ph_{nk}}
    +\frac{\partial \LM_f }{\partial \ph_{nk}}
    + \frac{\partial \LM_s }{\partial \ph_{nk}}
    \\
    =& \Psi(\gamma_k)-\Psi(\sum_{j=1}^{K} \gamma_j) -\frac{1}{2}(\e_{n}-\muu_k)^T\Si_k^{-1}(\e_{n}-\muu_k) - \log \vert \Si_k\vert^{1/2} \nonumber \\
  &  -\log\ph_{nk} + \frac{1}{N} (\sum_{j=1}^{C} y_{j} \et_j 
    -  \frac{\sum_{j=1} ^{C} \exp(\et^T_{j} \bar\ph_d  + (1/2)\et_j^T\Si_{d}\et_j)\et_j} {\sum_{j=1}^{C} \exp (\et^T_{j} \bar\ph_d + (1/2)\et_j^T\Si_{d}\et_j)})_k  \\
    &+ \frac{1}{N} (\bet^T \bar \ph'_d  - \frac{\sum_{f\in \DB_{-d}}\exp (\bet^T  (\bar \ph_d\bar\ph_f)  ) \cdot \bet^T \bar\ph_f} {\sum_{f\in \DB_{-d}}\exp (\bet^T (\bar\ph_d\bar\ph_f ))})_k
    -1 + \lambda,
\end{align}

where $\LM_u, \LM_f, \LM_s$ are unsupervised, relevance, and stability terms, respectively. 
%(ref DDPM classifier guidence, RLDA, etc.)

Setting the derivative to $0$, we have a closed-form update rules for $\ph$ as follows:
\begin{align}\label{eq:update_phi_app}
    \phi_{nk} \propto & \frac{1}{\vert \Si_k\vert^{1/2}} 
      \exp[\Psi(\gamma_{k})-\Psi(\sum_{k'=1}^K \gamma_{k'}) 
     -\frac{1}{2}(\e_{n}-\muu_k)^T\Si_k^{-1}(\e_{n}-\muu_k)\nonumberß\\ 
     &+ \frac{1}{N} (\sum_{j=1}^{C} y_{j} \et_j 
    -  \frac{\sum_{j=1} ^{C} \exp(\et^T_{j} \bar\ph  +(1/2)\et_j^T\Si_{d}\et_j)\et_j} {\sum_{j=1}^{C} \exp (\et^T_{j} \bar\ph + (1/2)\et_j^T\Si_{d}\et_j)}
    \\ &+\bet^T \bar \ph'_d  - \frac{\sum_{f\in \DB_{-d}}\exp (\bet^T  (\bar \ph_d\bar\ph_f)  ) \cdot \bet^T \bar\ph_f} {\sum_{f\in \DB_{-d}}\exp (\bet^T (\bar\ph_d\bar\ph_f ))})_k ].
\end{align}
For negative samples in the batch, use similar technique to update. \red{Note that inside brackets, first two terms are R loss, whereas last two terms are S loss. Here we consider use adaptive gradient update (such as adagrad/adam) instead of closed-form solution after basic solution for two additional loss}

for learning stability, try to use 2/3-layer MLP(e) instead of e, and backprop from ELBO.

for evaluation, use L2 normalize $||c'-c||/||c||$
